# Supplementary material for: Surface Second Harmonic Generation in Centrosymmetric Molecular Crystalline Materials: How Thick is the Surface?
Source: arXiv:2310.20297 source file (2024-01-11)
Supplement: Supplementary file 1 [file Surface_SHG_of_Molecular_Crystalline_Materials_SI.pdf]

# Supplementary Information: Multi-scale Modeling of Surface Second Harmonic Generation in Centrosymmetric Molecular Crystalline Materials: How Thick is the Surface?

Benedikt Zerulla,<sup>1</sup> Alejandro Luna Díaz,<sup>2</sup> Christof Holzer,<sup>2</sup> Carsten Rockstuhl,<sup>2,1</sup> Ivan Fernandez-Corbaton,<sup>1</sup> and Marjan Krstić<sup>2</sup>

<sup>1</sup>*Institute of Nanotechnology, Karlsruhe Institute of Technology (KIT), Kaiserstr. 12, 76131 Karlsruhe, Germany*

<sup>2</sup>*Institute of Theoretical Solid State Physics, Karlsruhe Institute of Technology (KIT), Kaiserstr. 12, 76131 Karlsruhe, Germany*

(Dated: 9 January 2024)

TABLE I: The DFT calculated NBO partial charges of atoms in the unit cell of Urea crystal used to build partial charges field for the embedding of the quantum region.

| Atom number | Atom type | NBO partial charge |
|-------------|-----------|--------------------|
| 1           | C         | 0.72301            |
| 2           | O         | -0.65349           |
| 3           | N         | -0.82519           |
| 4           | H         | 0.41547            |
| 5           | H         | 0.37573            |
| 6           | N         | -0.82519           |
| 7           | H         | 0.41547            |
| 8           | H         | 0.38705            |
| 9           | H         | 0.37573            |
| 10          | C         | 0.72817            |
| 11          | O         | -0.65932           |
| 12          | N         | -0.82624           |
| 13          | H         | 0.39796            |
| 14          | H         | 0.37911            |
| 15          | N         | -0.82136           |
| 16          | H         | 0.41307            |

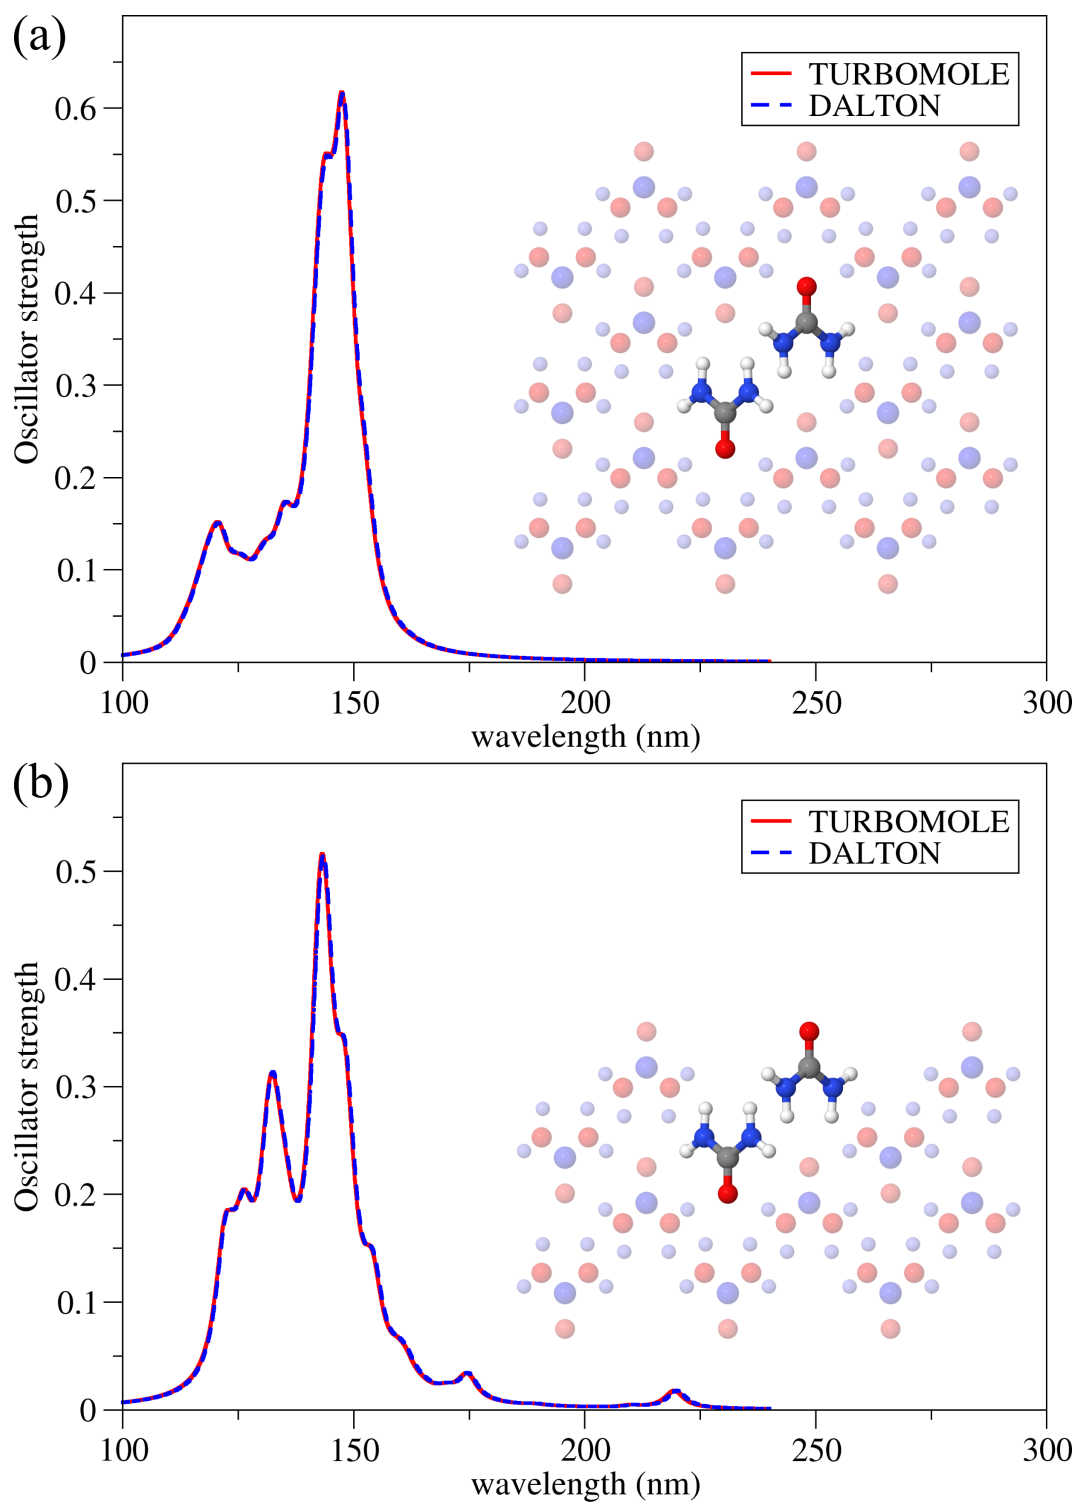

FIG. S1: **(a)** The OPA spectrum of urea bulk model calculated with TURBOMOLE and DALTON program. **(b)** The OPA spectrum of urea surface model calculated with TURBOMOLE and DALTON program.

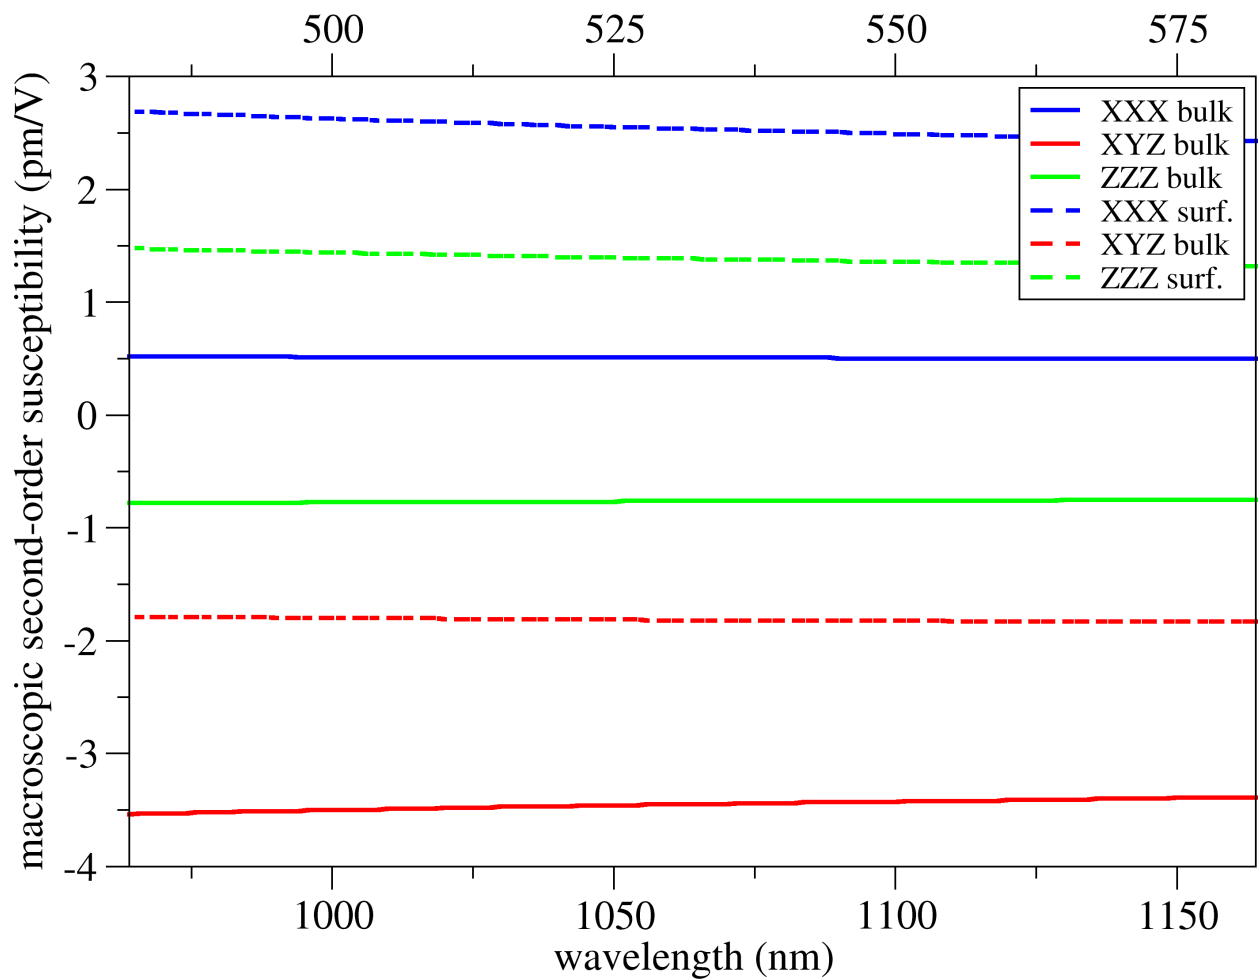

FIG. S2: Calculated macroscopic second-order susceptibility based on TD-DFT calculations and approach adapted from Miniewicz *et al.*<sup>1</sup>.

TABLE II: The DFT calculated NBO partial charges of atoms in the unit cell of the 7,9-Dibromobenzo[*h*]quinolin-10-ol crystal used to build partial charges field for the embedding of the quantum region.

| Atom number | Atom type | NBO partial charge |
|-------------|-----------|--------------------|
| 1           | Br        | 0.06966            |
| 2           | Br        | 0.05114            |
| 3           | O         | -0.65152           |
| 4           | H         | 0.50747            |
| 5           | N         | -0.45422           |
| 6           | C         | 0.30585            |
| 7           | C         | -0.13817           |
| 8           | C         | -0.20632           |
| 9           | H         | 0.2095             |
| 10          | C         | -0.0796            |
| 11          | C         | -0.06356           |
| 12          | C         | -0.14286           |
| 13          | H         | 0.19697            |
| 14          | C         | -0.15967           |
| 15          | H         | 0.19116            |
| 16          | C         | -0.07435           |
| 17          | C         | -0.10745           |
| 18          | H         | 0.19127            |
| 19          | C         | -0.2233            |
| 20          | H         | 0.19295            |
| 21          | C         | 0.10754            |
| 22          | H         | 0.18546            |
| 23          | C         | 0.1899             |
| 24          | C         | -0.10132           |
| 25          | Br        | 0.08166            |
| 26          | Br        | 0.05955            |
| 27          | O         | -0.63807           |
| 28          | H         | 0.50532            |
| 29          | N         | -0.45042           |
| 30          | C         | 0.30766            |
| 31          | C         | -0.13767           |
| 32          | C         | -0.21037           |
| 33          | H         | 0.20936            |
| 34          | C         | -0.08143           |
| 35          | C         | -0.06373           |
| 36          | C         | -0.13156           |
| 37          | H         | 0.19863            |
| 38          | C         | -0.16593           |
| 39          | H         | 0.19077            |
| 40          | C         | -0.0697            |

| Atom number | Atom type | NBO partial charge |
|-------------|-----------|--------------------|
| 41          | C         | -0.1079            |
| 42          | H         | 0.18838            |
| 43          | C         | -0.22441           |
| 44          | H         | 0.19258            |
| 45          | C         | 0.08897            |
| 46          | H         | 0.1735             |
| 47          | C         | 0.19099            |
| 48          | C         | -0.10268           |
| 49          | Br        | 0.06966            |
| 50          | Br        | 0.05097            |
| 51          | O         | -0.65149           |
| 52          | H         | 0.50748            |
| 53          | N         | -0.45416           |
| 54          | C         | 0.30618            |
| 55          | C         | -0.13844           |
| 56          | C         | -0.2059            |
| 57          | H         | 0.20944            |
| 58          | C         | -0.07953           |
| 59          | C         | -0.06388           |
| 60          | C         | -0.14275           |
| 61          | H         | 0.19695            |
| 62          | C         | -0.15971           |
| 63          | H         | 0.19116            |
| 64          | C         | -0.07423           |
| 65          | C         | -0.10746           |
| 66          | H         | 0.19126            |
| 67          | C         | -0.22333           |
| 68          | H         | 0.19295            |
| 69          | C         | 0.10757            |
| 70          | H         | 0.18546            |
| 71          | C         | 0.18959            |
| 72          | C         | -0.10126           |
| 73          | Br        | 0.08167            |
| 74          | Br        | 0.05936            |
| 75          | O         | -0.63806           |
| 76          | H         | 0.50533            |
| 77          | N         | -0.45044           |
| 78          | C         | 0.30767            |
| 79          | C         | -0.13767           |
| 80          | C         | -0.21008           |
| 81          | H         | 0.20931            |
| 82          | C         | -0.08122           |

| Atom number | Atom type | NBO partial charge |
|-------------|-----------|--------------------|
| 83          | C         | -0.06415           |
| 84          | C         | -0.13145           |
| 85          | H         | 0.19862            |
| 86          | C         | -0.16594           |
| 87          | H         | 0.19077            |
| 88          | C         | -0.06971           |
| 89          | C         | -0.10792           |
| 90          | H         | 0.18838            |
| 91          | C         | -0.22442           |
| 92          | H         | 0.19258            |
| 93          | C         | 0.08897            |
| 94          | H         | 0.1735             |
| 95          | C         | 0.19102            |
| 96          | C         | -0.10264           |

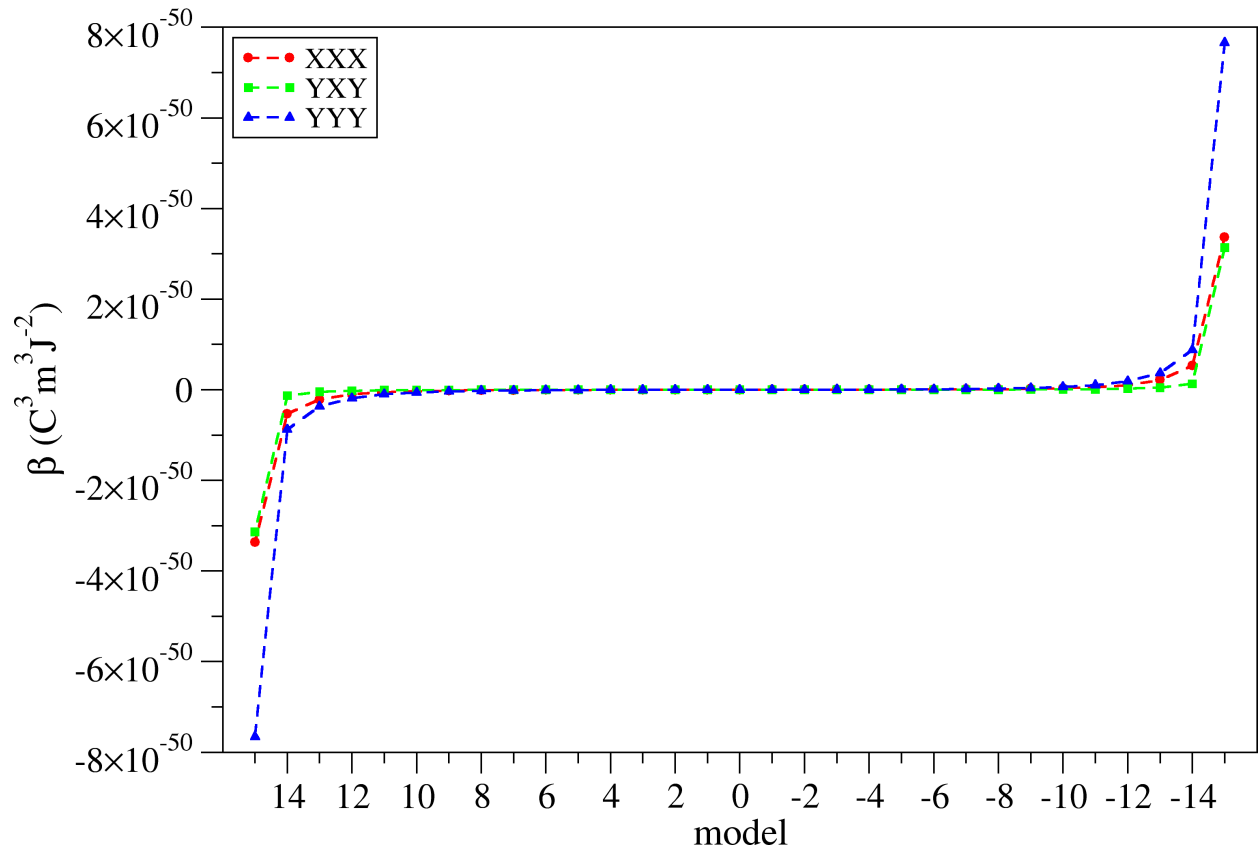

FIG. S3: The real part of calculated first-hyperpolarizabilities in SI units for the most prominent components of the tensor for models "-15" to "15".

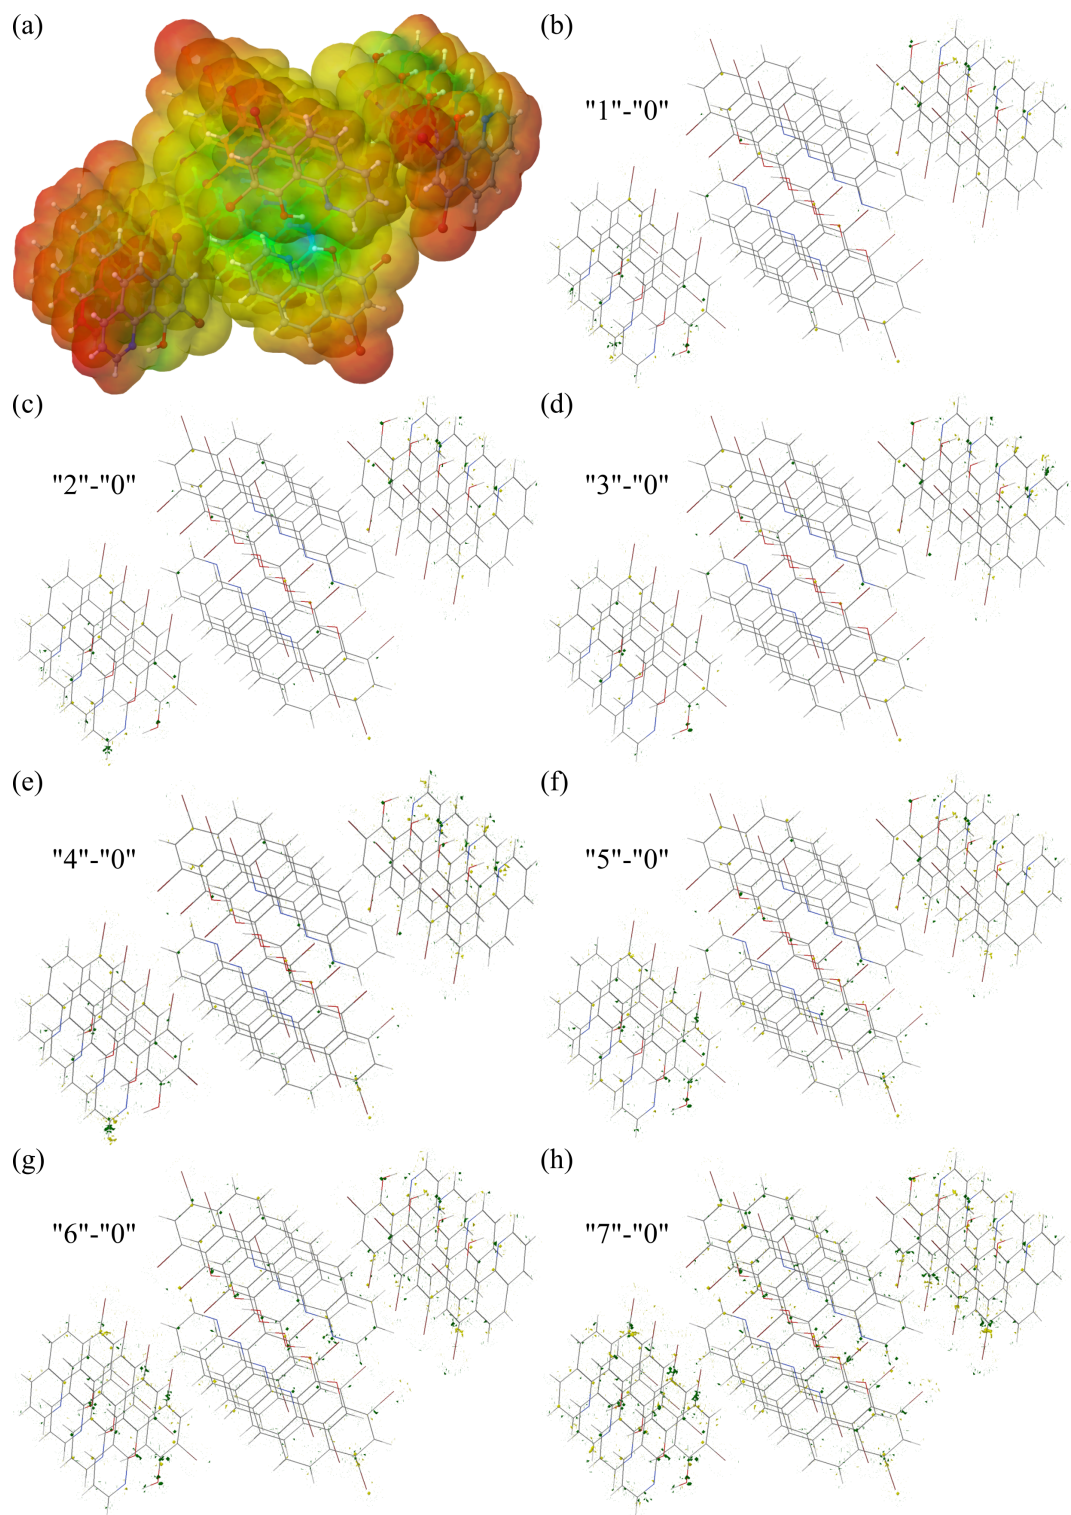

FIG. S4: **(a)** The electrostatic potential mapped on the total electron density. **(b-h)** The total electron density difference between models "1 to "7" and model "0". Green and yellow color represent positive and negative difference in total density, respectively. The isosurface is plotted for cutoff  $\pm 0.00001$ . This figure should be considered together with the Figure S5.

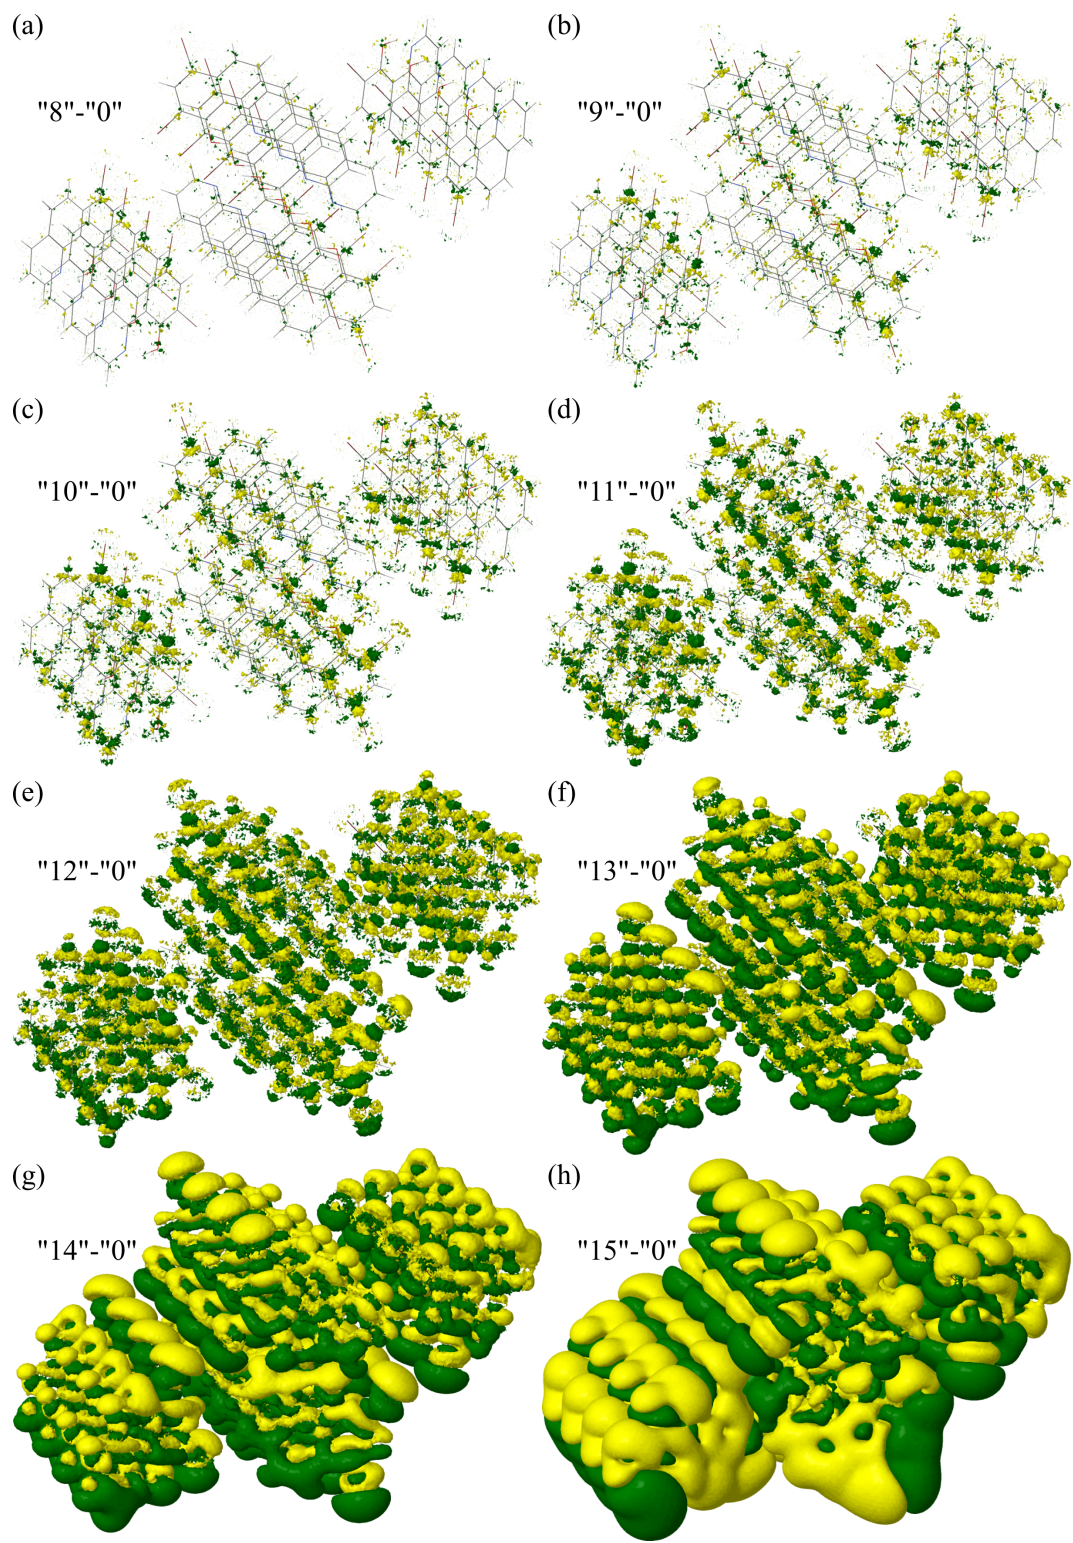

FIG. S5: **(a-h)** The total electron density difference between models "8" to "15" and model "0". Green and yellow color represent positive and negative difference in total density, respectively. The isosurface is plotted for cutoff  $\pm 0.00001$ . This figure should be considered together with the Figure S4.

TABLE III: The induced electronic dipole moment of the quantum models when approaching to the interfaces. The values are Cartesian components of dipole moments in Debyes. The induced moments are the largest at the surface.

| Model | x                      | y                      | z                     |
|-------|------------------------|------------------------|-----------------------|
| 15    | -2.921720482682428     | -4.58828086093882      | -2.9534262909932196   |
| 14    | -0.403970734172472     | -0.69096243869226      | -1.4125275655408398   |
| 13    | -0.165445147407228     | -0.285560698420784     | -0.64895999502256     |
| 12    | -0.078583331372836     | -0.143568292177872     | -0.32327266554497996  |
| 11    | -0.040421474231724     | -0.07990250040548799   | -0.175235974216044    |
| 10    | -0.025872488599932002  | -0.049348105527820006  | -0.10508109084373599  |
| 9     | -0.016091828797148     | -0.030478142332427998  | -0.067099698059692    |
| 8     | -0.009264684246659998  | -0.018572578268956     | -0.044025677870067996 |
| 7     | -0.008436073255052     | -0.014724366485844001  | -0.030661148441004    |
| 6     | -0.005241091609496     | -0.009706949009052     | -0.022362329767384    |
| 5     | -0.0037236659592199996 | -0.006173914412932     | -0.016755225940735998 |
| 4     | -0.001420839092972     | -0.002447706702204     | -0.010286468352876001 |
| 3     | -0.00163942972266      | -0.003944798340416     | -0.008006517250199999 |
| 2     | -0.000772692458432     | -0.0013572953052719999 | -0.005556268796488    |
| 1     | -0.000617645616444     | -7.1169042224e-05      | -0.002971307512852    |
| 0     | 0.0                    | 0.0                    | -0.0                  |
| -1    | 0.000617645616444      | 7.1169042224e-05       | 0.002971307512852     |
| -2    | 0.000772692458432      | 0.0013572953052719999  | 0.005556268796488     |
| -3    | 0.00163942972266       | 0.003944798340416      | 0.008006517250199999  |
| -4    | 0.001420839092972      | 0.002447706702204      | 0.010286468352876001  |
| -5    | 0.0037236659592199996  | 0.006173914412932      | 0.016755225940735998  |
| -6    | 0.005241091609496      | 0.009706949009052      | 0.022362329767384     |
| -7    | 0.008436073255052      | 0.014724366485844001   | 0.030661148441004     |
| -8    | 0.009264684246659998   | 0.018572578268956      | 0.044025677870067996  |
| -9    | 0.016091828797148      | 0.030478142332427998   | 0.067099698059692     |
| -10   | 0.025872488599932002   | 0.049348105527820006   | 0.10508109084373599   |
| -11   | 0.040421474231724      | 0.07990250040548799    | 0.175235974216044     |
| -12   | 0.078583331372836      | 0.143568292177872      | 0.32327266554497996   |
| -13   | 0.165445147407228      | 0.285560698420784      | 0.64895999502256      |
| -14   | 0.403970734172472      | 0.69096243869226       | 1.4125275655408398    |
| -15   | 2.921720482682428      | 4.58828086093882       | 2.9534262909932196    |

## REFERENCES

- <sup>1</sup>A. Miniewicz, S. Bartkiewicz, E. Wojaczynska, T. Galica, R. Zalesny, and R. Jakubas, “Second harmonic generation in nonlinear optical crystals formed from propellane-type molecules,” *J. Mater. Chem. C* **7**, 1255–1262 (2019).
